# Supplementary material for: Voiced-Aware Style Extraction and Style Direction Adjustment for Expressive Text-to-Speech
Source: arXiv:2511.14824 source file (2025-11-18)
Supplement: Supplementary file 1 [file appendices.tex]

% \input{chapters/appendix_codes}
